# Supplementary material for: Systematic Comparison and Cross-validation of Fixed-Node Diffusion Monte Carlo and Phaseless Auxiliary-Field Quantum Monte Carlo in Solids
Source: arXiv:2007.05587 ancillary file (2020-07-10)
Supplement: Supplementary file 1 [file supplement.pdf]

# Supplementary Material for ‘Systematic Comparison and Cross-validation of Fixed-Node Diffusion Monte Carlo and Phaseless Auxiliary-Field Quantum Monte Carlo in Solids’

Fionn D. Malone,[1,*] Anouar Benali,[2,*] Miguel A. Morales,[1]
Michel Caffarel,[3] P. R. C. Kent,[4] and Luke Shulenburger[5,†]

[1] *Quantum Simulations Group, Lawrence Livermore National Laboratory, 7000 East Avenue, Livermore, CA, 94551 USA.*

[2] *Argonne Leadership Computing Facility, Argonne National Laboratory, Argonne, Illinois 60439 USA*

[3] *Laboratoire de Chimie et Physique Quantiques, Université de Toulouse, CNRS, UPS, France*

[4] *Center for Nanophase Materials Sciences Division and Computational Sciences and Engineering Division, Oak Ridge National Laboratory, Oak Ridge, Tennessee 37831, USA.*

[5] *HEDP Theory Department, Sandia National Laboratories, Albuquerque, New Mexico 87185 USA*

## I. CIPSI CALCULATIONS

Below in Figs. (1)-(9) we plot the CIPSI variational energy, $E_{\mathrm{var}}$, as a function of the second-order correction energy, $E_{\mathrm{PT2}}$, for the systems studied in the main text. The extrapolated CIPSI variational energy at the origin, $E_{\mathrm{PT2}} = 0$, is an estimate of the FCI energy within the finite basis set labeled as exFCI. The values for the exFCI energies are reported in Table I.

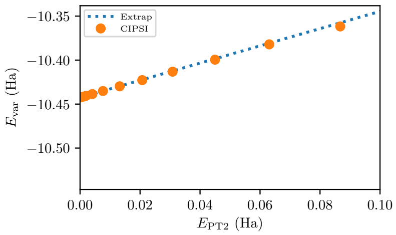


FIG. 1. C (Diamond) cc-pVDZ

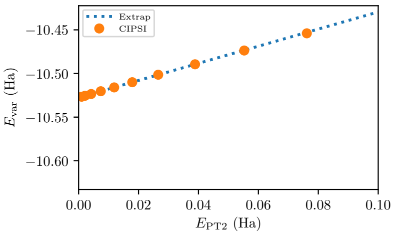


FIG. 2. C (Diamond) cc-pVTZ

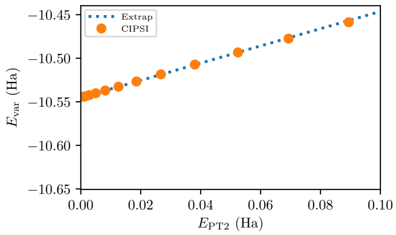


FIG. 3. C (Diamond) cc-pVQZ

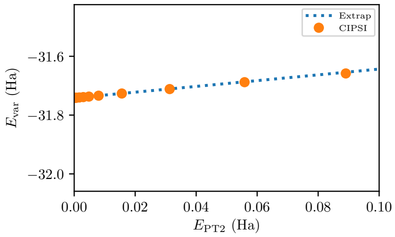


FIG. 4. LiF cc-pVDZ

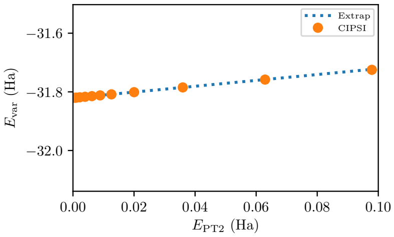


FIG. 5. LiF cc-pVTZ

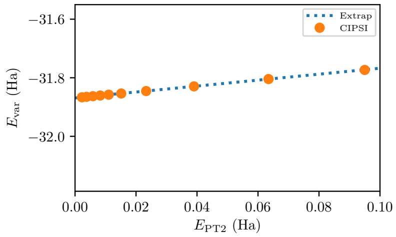


FIG. 6. LiF cc-pVQZ

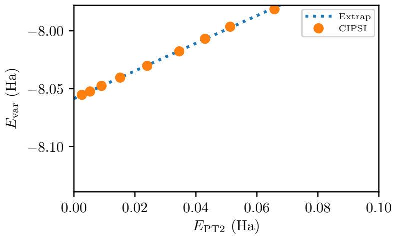


FIG. 7. Al cc-pVDZ

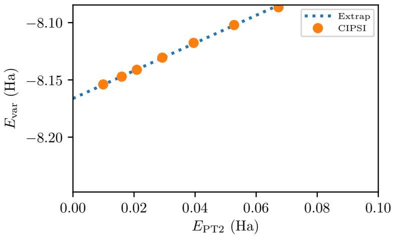


FIG. 8. Al cc-pVTZ

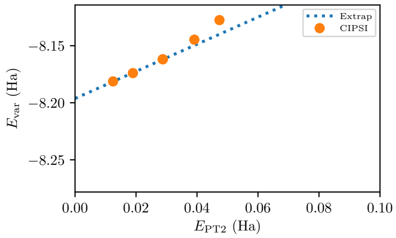


FIG. 9. Al cc-pVQZ

| system | basis | Nb Det | $E_{\mathrm{PT2}}$ | $E_{var}$ | exFCI |
|---|---|---|---|---|---|
| C (Diamond) | DZ | 1452156 | 0.0003 | -10.442236 | -10.442585 |
| | TZ | 5334449 | 0.0010 | -10.526609 | -10.527608 |
| | QZ | 16446929 | 0.0009 | -10.545157 | -10.545158 |
| LiF | DZ | 713884 | 0.0002 | -31.741420 | -31.741690 |
| | TZ | 6108137 | 0.0005 | -31.820213 | -31.820796 |
| | QZ | 9753780 | 0.0023 | -31.866668 | -31.868958 |
| Al | DZ | 5395686 | 0.0026 | -8.055291 | -8.058480 |
| | TZ | 7808133 | 0.0099 | -8.153964 | -8.166251 |
| | QZ | 12488536 | 0.0125 | -8.181255 | -8.196254 |

TABLE I. CIPSI variational energies and second-order energy corrections for all systems studied and basis sets used. The total number of determinants considered in each expansion is also reported. exFCI energies are obtained by extrapolating the CIPSI variational energies at $E_{\mathrm{PT2}} = 0$ as explained in the main text. Energies are in Hartree atomic units.

### A. Basis Set Extrapolation

To obtain CBS-limit exFCI total energies we extrapolated the exFCI correlation energy using the usual form[1]

$$E_c(X) = E_c(\infty) + BX^{-3}, \tag{1}$$

where $X$ is the cardinality of the basis set. We used a two-point extrapolation with $X =$T, Q. Here $E_c(X) = E(X) - E_{\mathrm{HF}}(X)$, where $E(X)$ and $E_{\mathrm{HF}}(X)$ are the exFCI and Hartree–Fock energies in basis set $X$, respectively. The Hartree–Fock energies were separately extrapolated using an exponential form[1] using $X$=D,T,Q. Extrapolating with T,Q,5 lead to indistinguishable results for Diamond. In Figs. (13)-(16) we plot the extrapolation of the correlation energy

| system | basis | Energy (Ha/Cell) |
|---|---|---|
| LiF | DZ | -31.55100 |
| | TZ | -31.55438 |
| | QZ | -31.55543 |
| | $\infty$ | -31.55590 |
| Diamond | DZ | -10.21255 |
| | TZ | -10.23639 |
| | QZ | -10.23801 |
| | 5Z | -10.23812 |
| | $\infty$ | -10.23814 |
| Al | DZ | -7.76040 |
| | TZ | -7.79213 |
| | QZ | -7.79756 |
| | $\infty$ | -7.79868 |

TABLE II. Hartree–Fock energies for different basis set sizes for the systems studied in the main text. Energies were computed using PySCF[2] with basis sets and ECPs from Refs. 3,4.

performed. In Table III we summarize our CBS-limit values for the HF, exFCI, and correlation energies.

| System | CBS-$E_{\mathrm{HF}}$ | CBS-$E_{\mathrm{exFCI}}$ | CBS-$E_c$ |
|---|---|---|---|
| C (Diamond) | -10.2381 | -10.5569 | -0.3188 |
| LiF | -31.5559 | -31.9038 | -0.3479 |
| Al | -7.7987 | -8.2153 | -0.4166 |

TABLE III. CBS-limit values for Hartree-Fock, exFCI, and corresponding exact correlation energies. Energies are in Hartree atomic units.

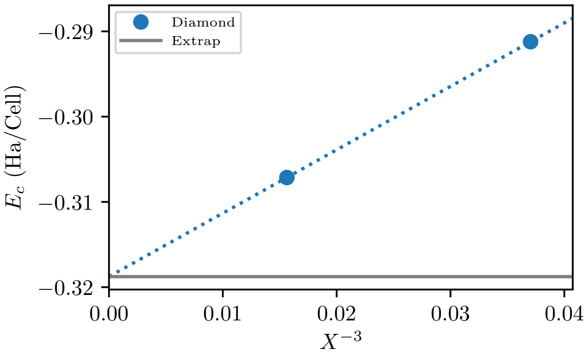


FIG. 10. CIPSI Diamond basis set extrapolation.

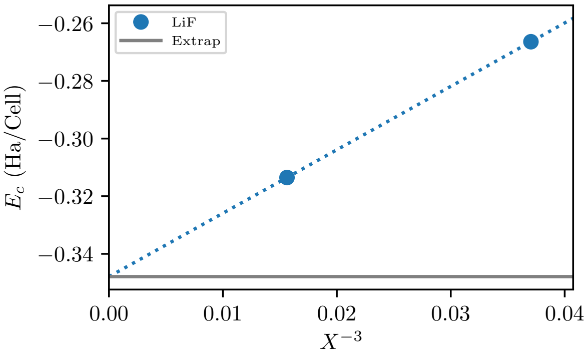


FIG. 11. CIPSI LiF basis set extrapolation.

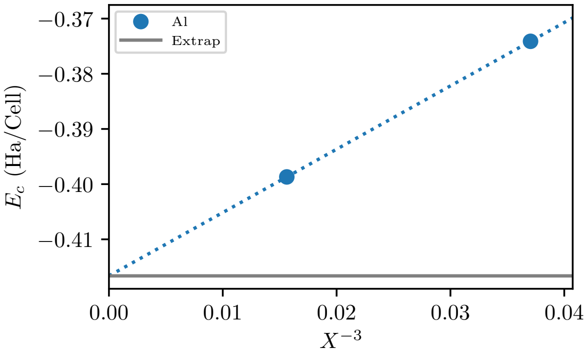


FIG. 12. CIPSI Al basis set extrapolation.

## II. AFQMC CALCULATIONS

The raw AFQMC total energies with different lengths of CIPSI trial wavefunctions are presented in Table IV.

### A. Basis Sets

The AFQMC basis set extrapolation procedure is identical to that as was used in the CIPSI calculations. In Figs. (17)-(20) we plot the AFQMC CBS extrapolations for two different trial wavefunction expansion lengths ($N_{\mathrm{Det}} = (1, 1000)$). These two points make up the AFQMC results in the main figure of the text. In Table V we present the AFQMC CBS total energies.

## III. DMC CONVERGENCE

The raw DMC total energies with different lengths of CIPSI trial wavefunctions are presented in Table VI.

| system | basis | $N_D$ | E(AFQMC) |
|---|---|---|---|
| Diamond | DZ | 1 | -10.4352(5) |
| | | 100 | -10.4410(2) |
| | | 500 | -10.44176(6) |
| | | 1000 | -10.44194(4) |
| Diamond | TZ | 1 | -10.5205(5) |
| | | 100 | -10.5258(2) |
| | | 500 | -10.5267(1) |
| | | 1000 | -10.5267(1) |
| Diamond | QZ | 1 | -10.5377(5) |
| | | 10 | -10.5413(2) |
| | | 500 | -10.5443(2) |
| | | 1000 | -10.5443(2) |
| LiF | DZ | 1 | -31.7420(2) |
| | | 10 | -31.7422(2) |
| | | 50 | -31.7418(1) |
| | | 100 | -31.74191(8) |
| | | 500 | -31.74169(4) |
| | | 1000 | -31.74167(3) |
| LiF | TZ | 1 | -31.8213(3) |
| | | 10 | -31.8212(2) |
| | | 50 | -31.8210(2) |
| | | 100 | -31.8209(1) |
| | | 500 | -31.8208(1) |
| | | 1000 | -31.8208(2) |
| LiF | QZ | 1 | -31.8696(3) |
| | | 10 | -31.8694(2) |
| | | 50 | -31.8690(1) |
| | | 100 | -31.8690(1) |
| | | 500 | -31.8693(4) |
| | | 1000 | -31.8685(4) |
| Al | DZ | 1 | -8.0464(8) |
| | | 10 | -8.0485(5) |
| | | 100 | -8.0519(3) |
| | | 1000 | -8.0547(1) |
| Al | TZ | 1 | -8.1536(5) |
| | | 10 | -8.1553(3) |
| | | 100 | -8.1581(2) |
| | | 1000 | -8.1610(3) |
| Al | QZ | 1 | -8.1834(4) |
| | | 410 | -8.1899(2) |
| | | 692 | -8.1897(2) |
| | | 1137 | -8.1902(3) |

TABLE IV. ph-AFQMC total energies for systems studied in main text including data for different multi-determinant expansion length ($N_D$). Energies are in Hartree atomic units.

| system | $E_{\mathrm{HF}}$ | $N_D$ | Energy | $E_c$ |
|---|---|---|---|---|
| Diamond | -10.2381 | 1 | -10.5492(9) | -0.3110(9) |
| | | 1000 | -10.5561(3) | -0.3180(3) |
| LiF | -31.5559 | 1 | -31.9046(5) | -0.3487(5) |
| | | 1000 | -31.9030(7) | -0.3471(7) |
| Al | -7.7987 | 1 | -8.2022(8) | -0.4035(8) |
| | | 1137 | -8.2087(6) | -0.4100(6) |

TABLE V. Basis set extrapolated ph-AFQMC total energies using different length of multi determinant expansion ($N_{\mathrm{Det}}$). Error bars are in the last digit and account for systematic and statistical errors. Energies are in Hartree atomic units.

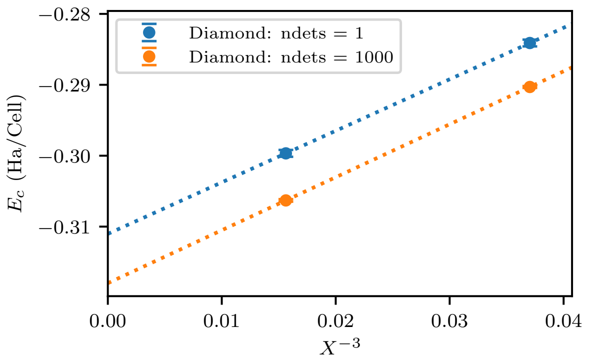


FIG. 13. Diamond basis set extrapolation.

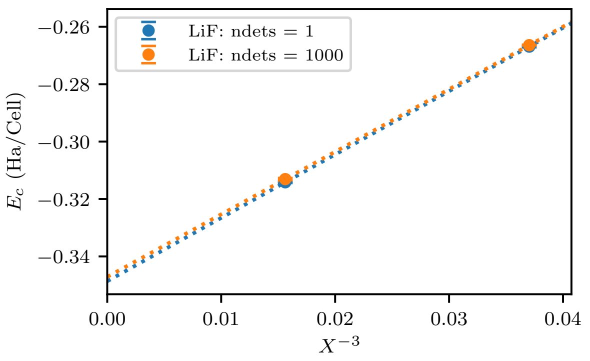


FIG. 14. LiF basis set extrapolation.

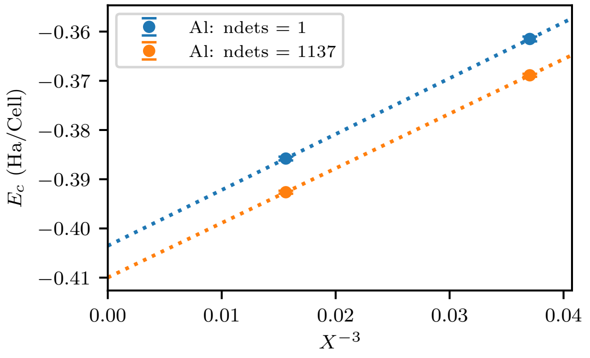


FIG. 15. Al basis set extrapolation.

| system | basis | Truncation | $N_D$ | E(DMC) |
|---|---|---|---|---|
| Diamond | DZ | - | 1 | -10.492102 (754) |
| | | $10^{-4}$ | 41470 | -10.528425 (213) |
| | | $10^{-5}$ | 368626 | -10.528632 (232) |
| | | $10^{-6}$ | 1110524 | -10.528807 (397) |
| | | $10^{-8}$ | 1442620 | -10.529382 (438) |
| Diamond | TZ | - | 1 | -10.499844 (530) |
| | | $10^{-2}$ | 166 | -10.531466 (199) |
| | | $10^{-3}$ | 1421147 | -10.537883 (184) |
| | | $10^{-4}$ | 83880 | -10.546763 (174) |
| | | $10^{-5}$ | 1421147 | -10.549715 (341) |
| | | $10^{-6}$ | 4474949 | -10.550193 (616) |
| | | $10^{-8}$ | 5316229 | -10.549240 (685) |
| Diamond | QZ | - | 1 | -10.500269 (577) |
| | | $10^{-4}$ | 90829 | -10.548301 (165) |
| | | $10^{-5}$ | 1650529 | -10.552679 (253) |
| | | $10^{-6}$ | 11269420 | -10.552397 (364) |
| | | $10^{-8}$ | 16144126 | -10.552626 (890) |
| LiF | DZ | - | 1 | -31.882034 (471) |
| | | $10^{-4}$ | 15375 | -31.887991 (251) |
| | | $10^{-5}$ | 210356 | -31.889049 (309) |
| | | $10^{-6}$ | 562143 | -31.888052 (372) |
| | | $10^{-8}$ | 708607 | -31.888795 (498) |
| LiF | TZ | - | 1 | -31.884306 (584) |
| | | $10^{-4}$ | 31383 | -31.893949 (220) |
| | | $10^{-5}$ | 730401 | -31.896634 (396) |
| | | $10^{-6}$ | 4282167 | -31.896897 (580) |
| | | $10^{-8}$ | 6043533 | -31.896512 (485) |
| LiF | QZ | - | 1 | -31.885199 (636) |
| | | $10^{-4}$ | 61035 | -31.888008 (247) |
| | | $10^{-5}$ | 1337151 | -31.889030 (308 |
| | | $10^{-6}$ | 7197124 | -31.89643 (105) |
| | | $10^{-8}$ | 9619883 | -31.896257 (918) |
| Al | DZ | - | 1 | -8.136132 (808) |
| | | $10^{-4}$ | 198380 | -8.168372 (350) |
| | | $10^{-5}$ | 926970 | -8.168113 (887) |
| | | $10^{-6}$ | 1226578 | -8.166912 (699) |
| | | $10^{-8}$ | 1324762 | -8.169838 (653) |
| Al | TZ | - | 1 | -8.151891 (789) |
| | | $10^{-4}$ | 297944 | -8.189657 (290) |
| | | $10^{-5}$ | 4038041 | -8.193273 (384) |
| | | $10^{-6}$ | 6702265 | -8.194089 (940) |
| Al | QZ | - | 1 | -8.164392 (707) |
| | | $10^{-4}$ | 335152 | -8.193251 (345) |
| | | $10^{-5}$ | 5771440 | -8.196837 (966) |
| | | $10^{-6}$ | 10524382 | -8.197836 (561) |

TABLE VI. DMC total energies for systems studied in main text including data for different multi-determinant expansion length ($N_D$). Energies are in Hartree atomic units.

* These authors contributed equally
† lshulen@sandia.gov

[1] T. Helgaker, W. Klopper, H. Koch, and J. Noga, J. Chem. Phys. **106**, 9639 (1997).
[2] Q. Sun, T. C. Berkelbach, N. S. Blunt, G. H. Booth, S. Guo, Z. Li, J. Liu, J. D. McClain, E. R. Sayfutyarova, S. Sharma, S. Wouters, and G. K. L. Chan, WIREs Comput. Mol. Sci. **8**, e1340 (2017).
[3] M. C. Bennett, C. A. Melton, A. Annaberdiyev, G. Wang, L. Shulenburger, and L. Mitas, The Journal of Chemical Physics **147**, 224106 (2017), https://doi.org/10.1063/1.4995643.
[4] M. C. Bennett, G. Wang, A. Annaberdiyev, C. A. Melton, L. Shulenburger, and L. Mitas, The Journal of Chemical Physics **149**, 104108 (2018).
